# Supplementary material for: Detail-Preserving Latent Diffusion for Stable Shadow Removal
Source: arXiv:2412.17630 source file (2024-12-23)
Supplement: Supplementary file 1 [file X_suppl.tex]

\clearpage

\setcounter{section}{0}
\setcounter{figure}{0}
\setcounter{table}{0}
\setcounter{page}{1}

\title{\vspace{-0.5em}-- Supplementary Material --\\Detail-Preserving Latent Diffusion for Stable Shadow Removal}

% \maketitlesupplementary
\maketitle

\noindent{In the supplementary material we present the following:}
\begin{itemize}%[topsep=3pt]
    \item Additional implementation details.
    \item Additional experiments and ablations.
\end{itemize}

\section{Additional Implementation Details}  
\label{sec:imp}

In our approach, we utilize Stable Diffusion v2~\cite{rombach2022high} in Diffusers~\cite{von-platen-etal-2022-diffusers}, setting the text prompt to an empty string for both training and testing phases. During the LDM fine-tuning stage (stage one), we adapt the U-Net by increasing its input channels from 4 to 8. These 8 channels include 4 for noise and 4 for the latent representation of the conditioning image. The additional parameters in the first layer are initialized by duplicating the original parameters and downscaling them by a factor of 2.

To adapt our method for large-size inputs, such as those in the WSRD+ dataset ($1920 \times 1440$), we make slight modifications to our two-stage approach. In the first stage, the input images are downscaled to $W/k \times H/k$, with $k=3$ for the WSRD+ dataset. We use smaller images in this stage to ensure high-quality shadow removal, accepting some loss of detail while prioritizing the capture of global contextual information. As a result, we resize the images rather than cropping them into local patches.

In the second stage, the input consists of the latent generated from the downscaled image in the first stage. The original image of shape $W \times H \times C$ is first reshaped to $\frac{W}{k} \times \frac{H}{k} \times Ck^2$, where the features of each $k \times k$ region are flattened into a vector. Using the VAE decoder with our Detail Injection model, the output is a feature map of shape $\frac{W}{k} \times \frac{H}{k} \times Ck^2$, which is then reshaped to the original dimensions, resulting in a large-size shadow-free image. Here, the input and output channels of the VAE are expanded from 3 to $3k^2$. The additional parameters in the first and last layers are initialized by duplicating and downscaling the original parameters. With this design, the features from the VAE encoder capture details from the large-size image, which are then injected into the decoder through the RRDB network to enhance its detail recovery. During training on the WRSD+ dataset~\cite{vasluianu2023wsrd}, we use 400 epochs for the first stage and 100 epochs for the second stage, with a batch size of 16. The results, presented in Fig.~\ref{fig:wrsd+}, demonstrate that our method effectively removes both hard and soft shadows from the high-resolution images.

\begin{figure}[t!]
\centering
\includegraphics[width=1.0\linewidth]{./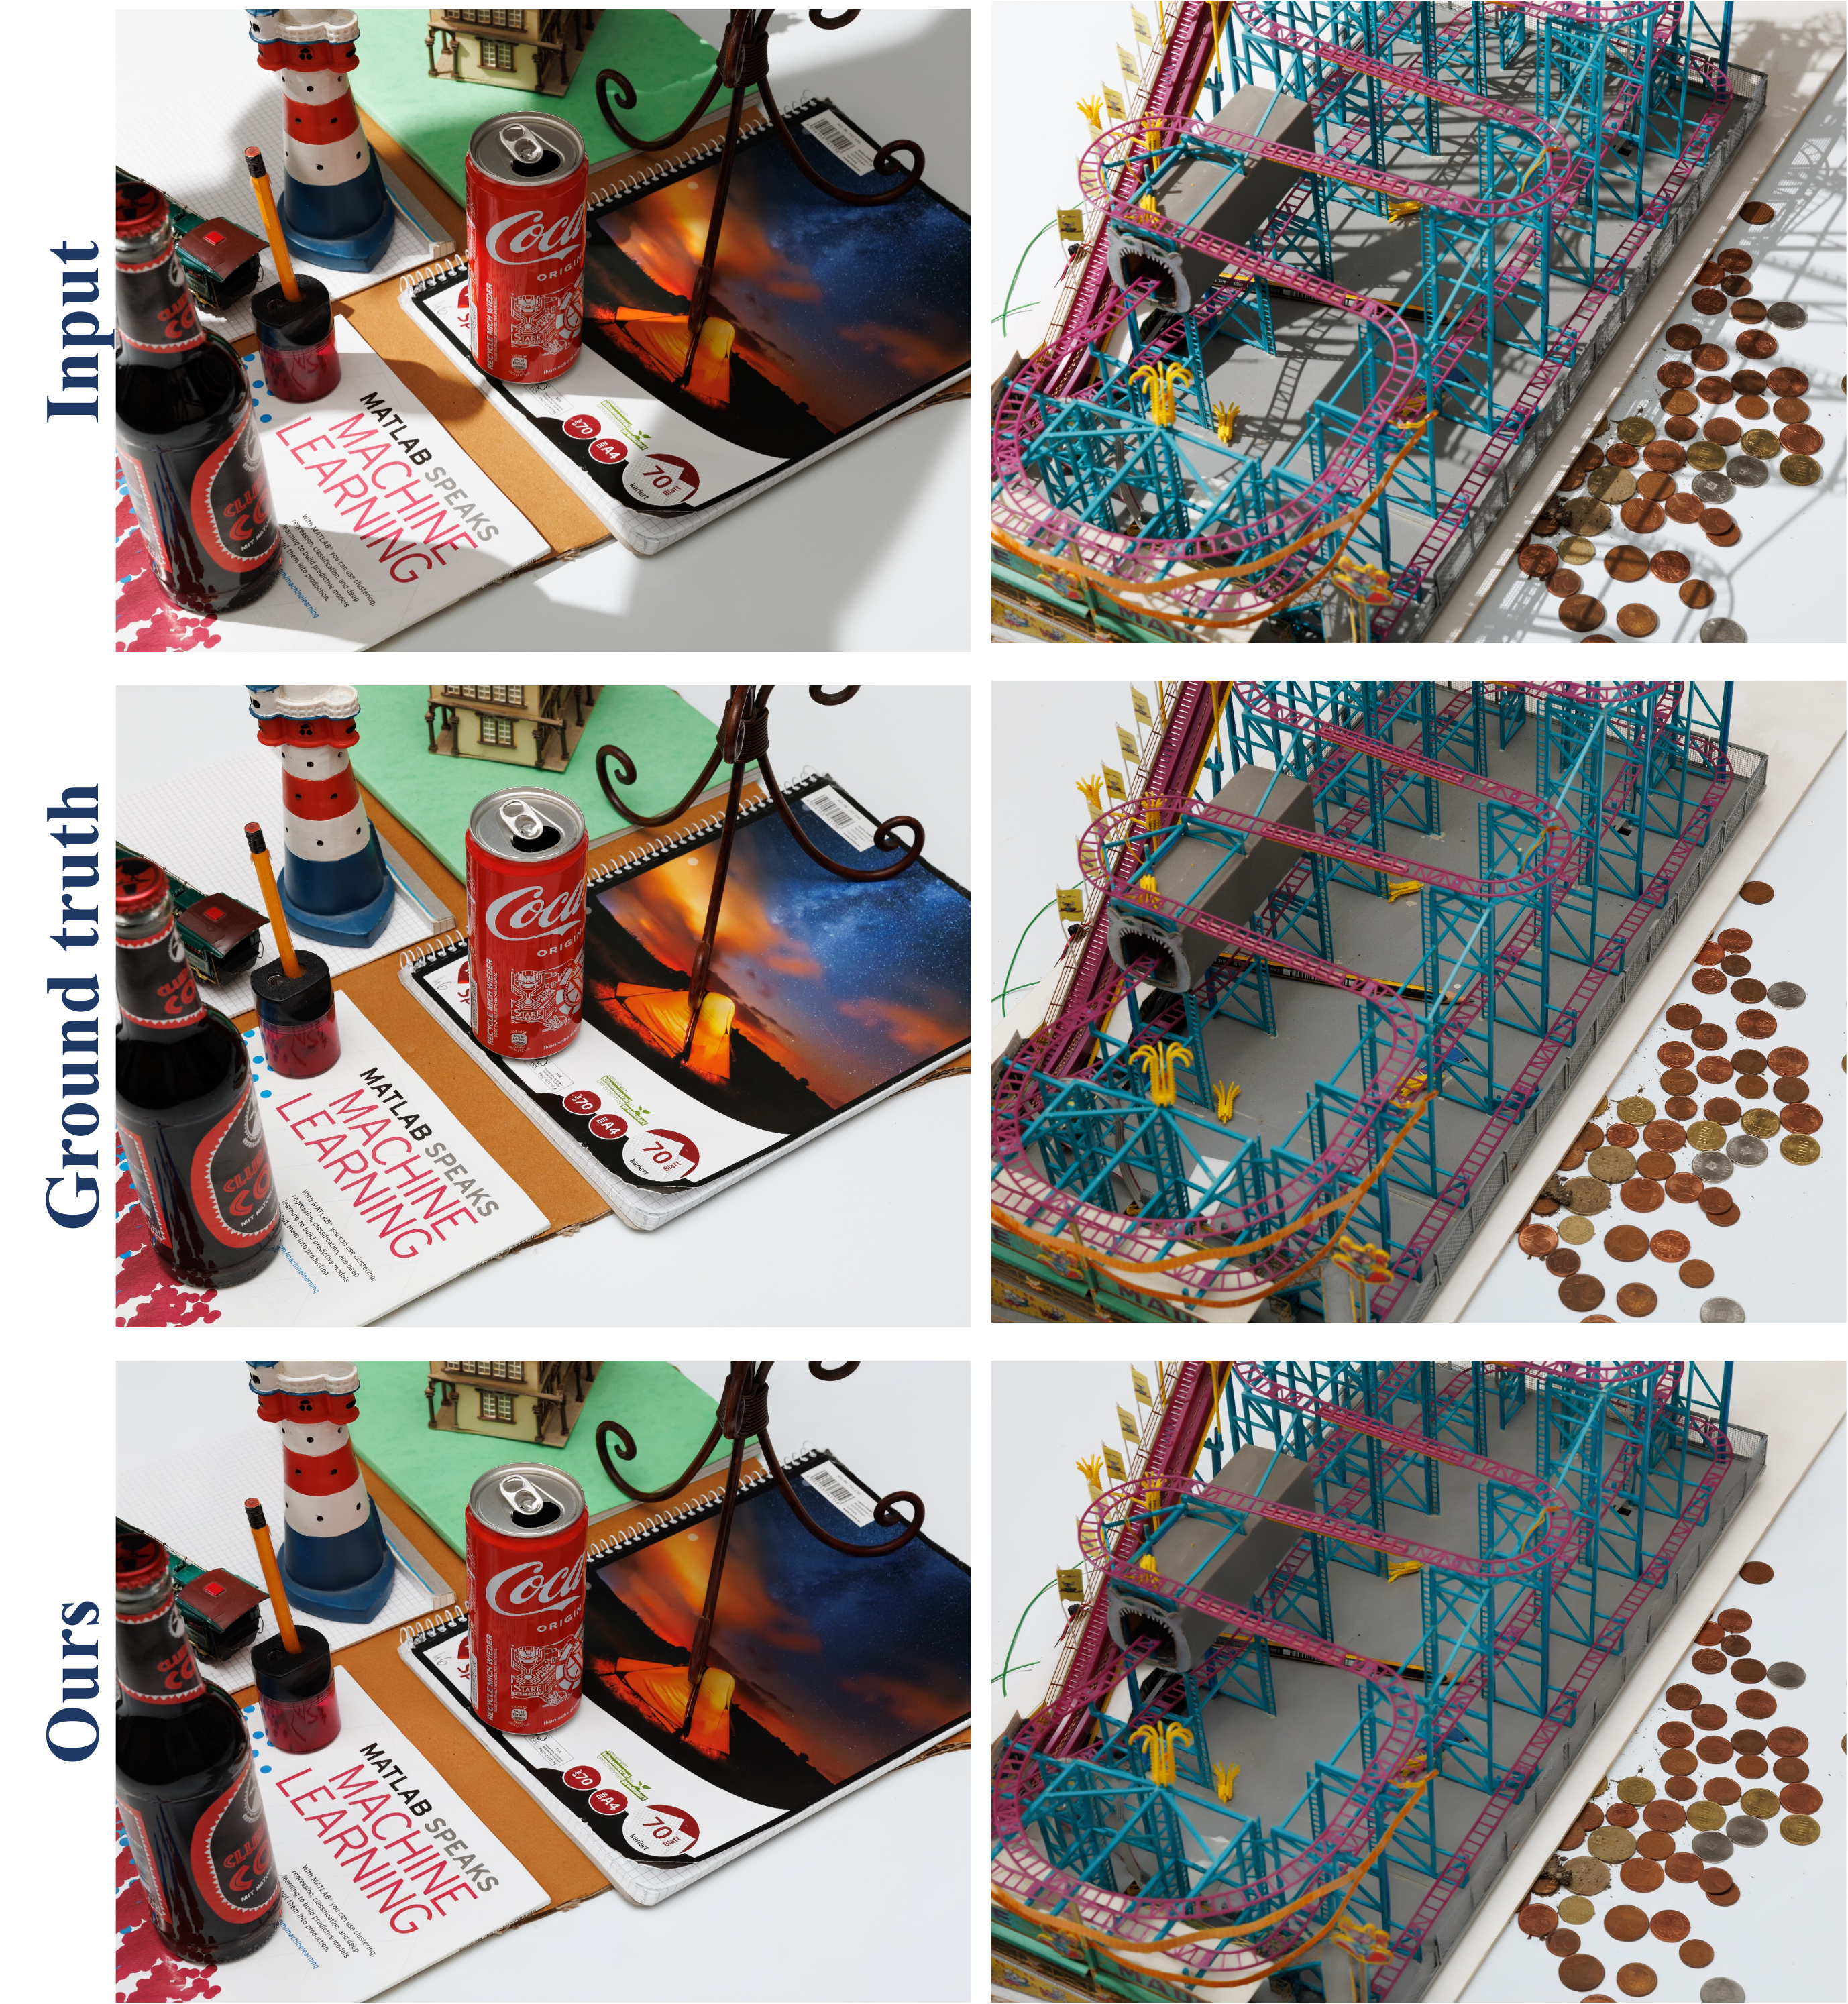}
\caption{\textbf{Our results on large-size inputs from the WSRD+ dataset ($1920 \times 1440$).}}
\label{fig:wrsd+} 
\end{figure}

\begin{figure*}[t!]
\centering
\includegraphics[width=1.0\linewidth]{./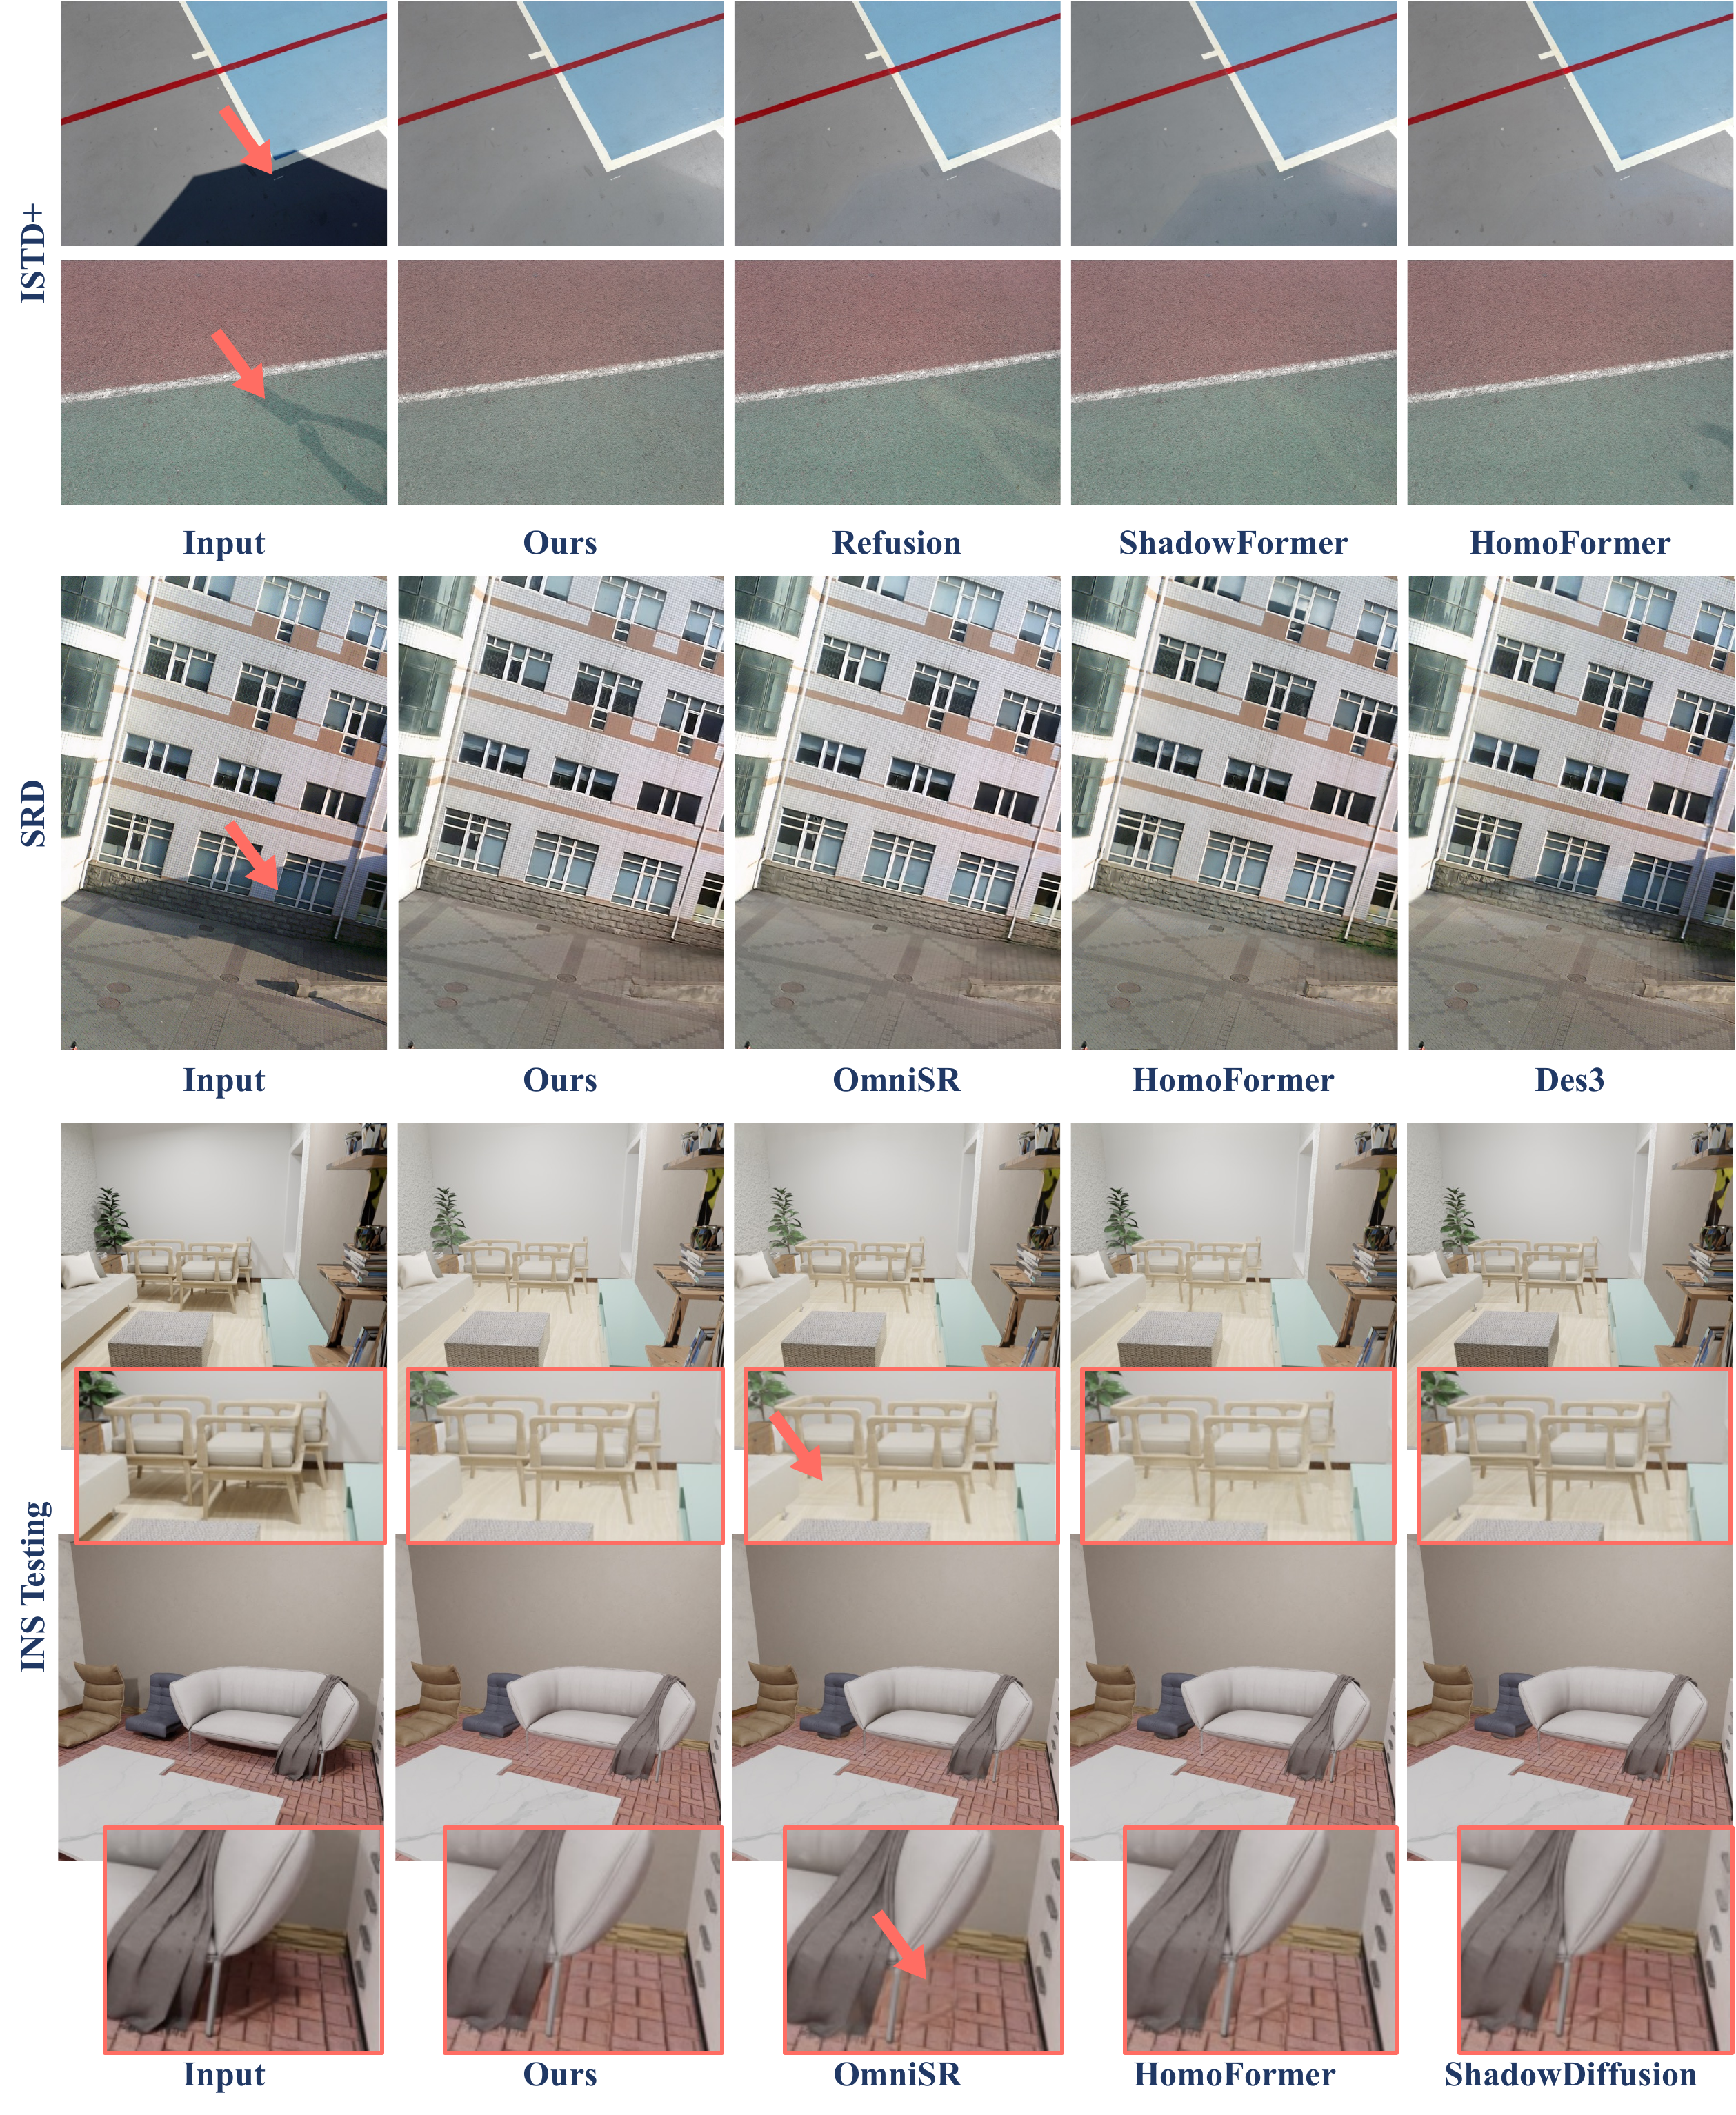}
\caption{\textbf{Additional comparison results on the ISTD+~\cite{le2019shadow}, SRD~\cite{qu2017deshadownet}, and INS dataset~\cite{xu2024omnisr}.}}
\label{fig:supp_comparison} 
\end{figure*}

\section{Additional Experiments and Ablations}  
\label{sec:add_exp}

\subsection{More results on the ISTD+~\cite{le2019shadow}, SRD~\cite{qu2017deshadownet}, and INS dataset~\cite{xu2024omnisr}}

In this section, we present the comparison results on the ISTD+~\cite{le2019shadow}, SRD~\cite{qu2017deshadownet}, and INS~\cite{xu2024omnisr} datasets in Fig.~\ref{fig:supp_comparison}. Our shadow removal method outperforms others, including those that rely on detected shadow masks, such as HomoFormer~\cite{xiao2024homoformer} and ShadowDiffusion~\cite{guo2023shadowdiffusion}, as well as methods that do not require shadow masks, such as Refusion~\cite{luo2023refusion}, Des3~\cite{jin2024des3}, and OmniSR~\cite{xu2024omnisr}. As shown in Fig.~\ref{fig:supp_comparison}, in the outdoor dataset, our method successfully removes hard shadows. 
In the INS~\cite{xu2024omnisr} indoor dataset, our method effectively removes complex shadows, such as those under the table and the thin shadow near the sofa.

\subsection{More results from our first and second stages}

We present additional results from the first and second stages, along with the colored RRDB features of different detail injection models, spanning from decoder layer one to four. As shown in Fig.~\ref{fig:rrdb_vis}, whether in outdoor or indoor settings, our detail injection model successfully injects shadow-free details into the decoder outputs, leading to shadow removal results that preserve intricate details. Additionally, by visualizing the RRDB features using PCA, we observe that shadow regions exhibit distinct colors compared to the surrounding areas. This suggests that the detail injection model in the second stage is able to learn to locate and remove shadows with the aid of the latent features from the first stage.

\begin{figure*}[t!]
\centering
\includegraphics[width=1.0\linewidth]{./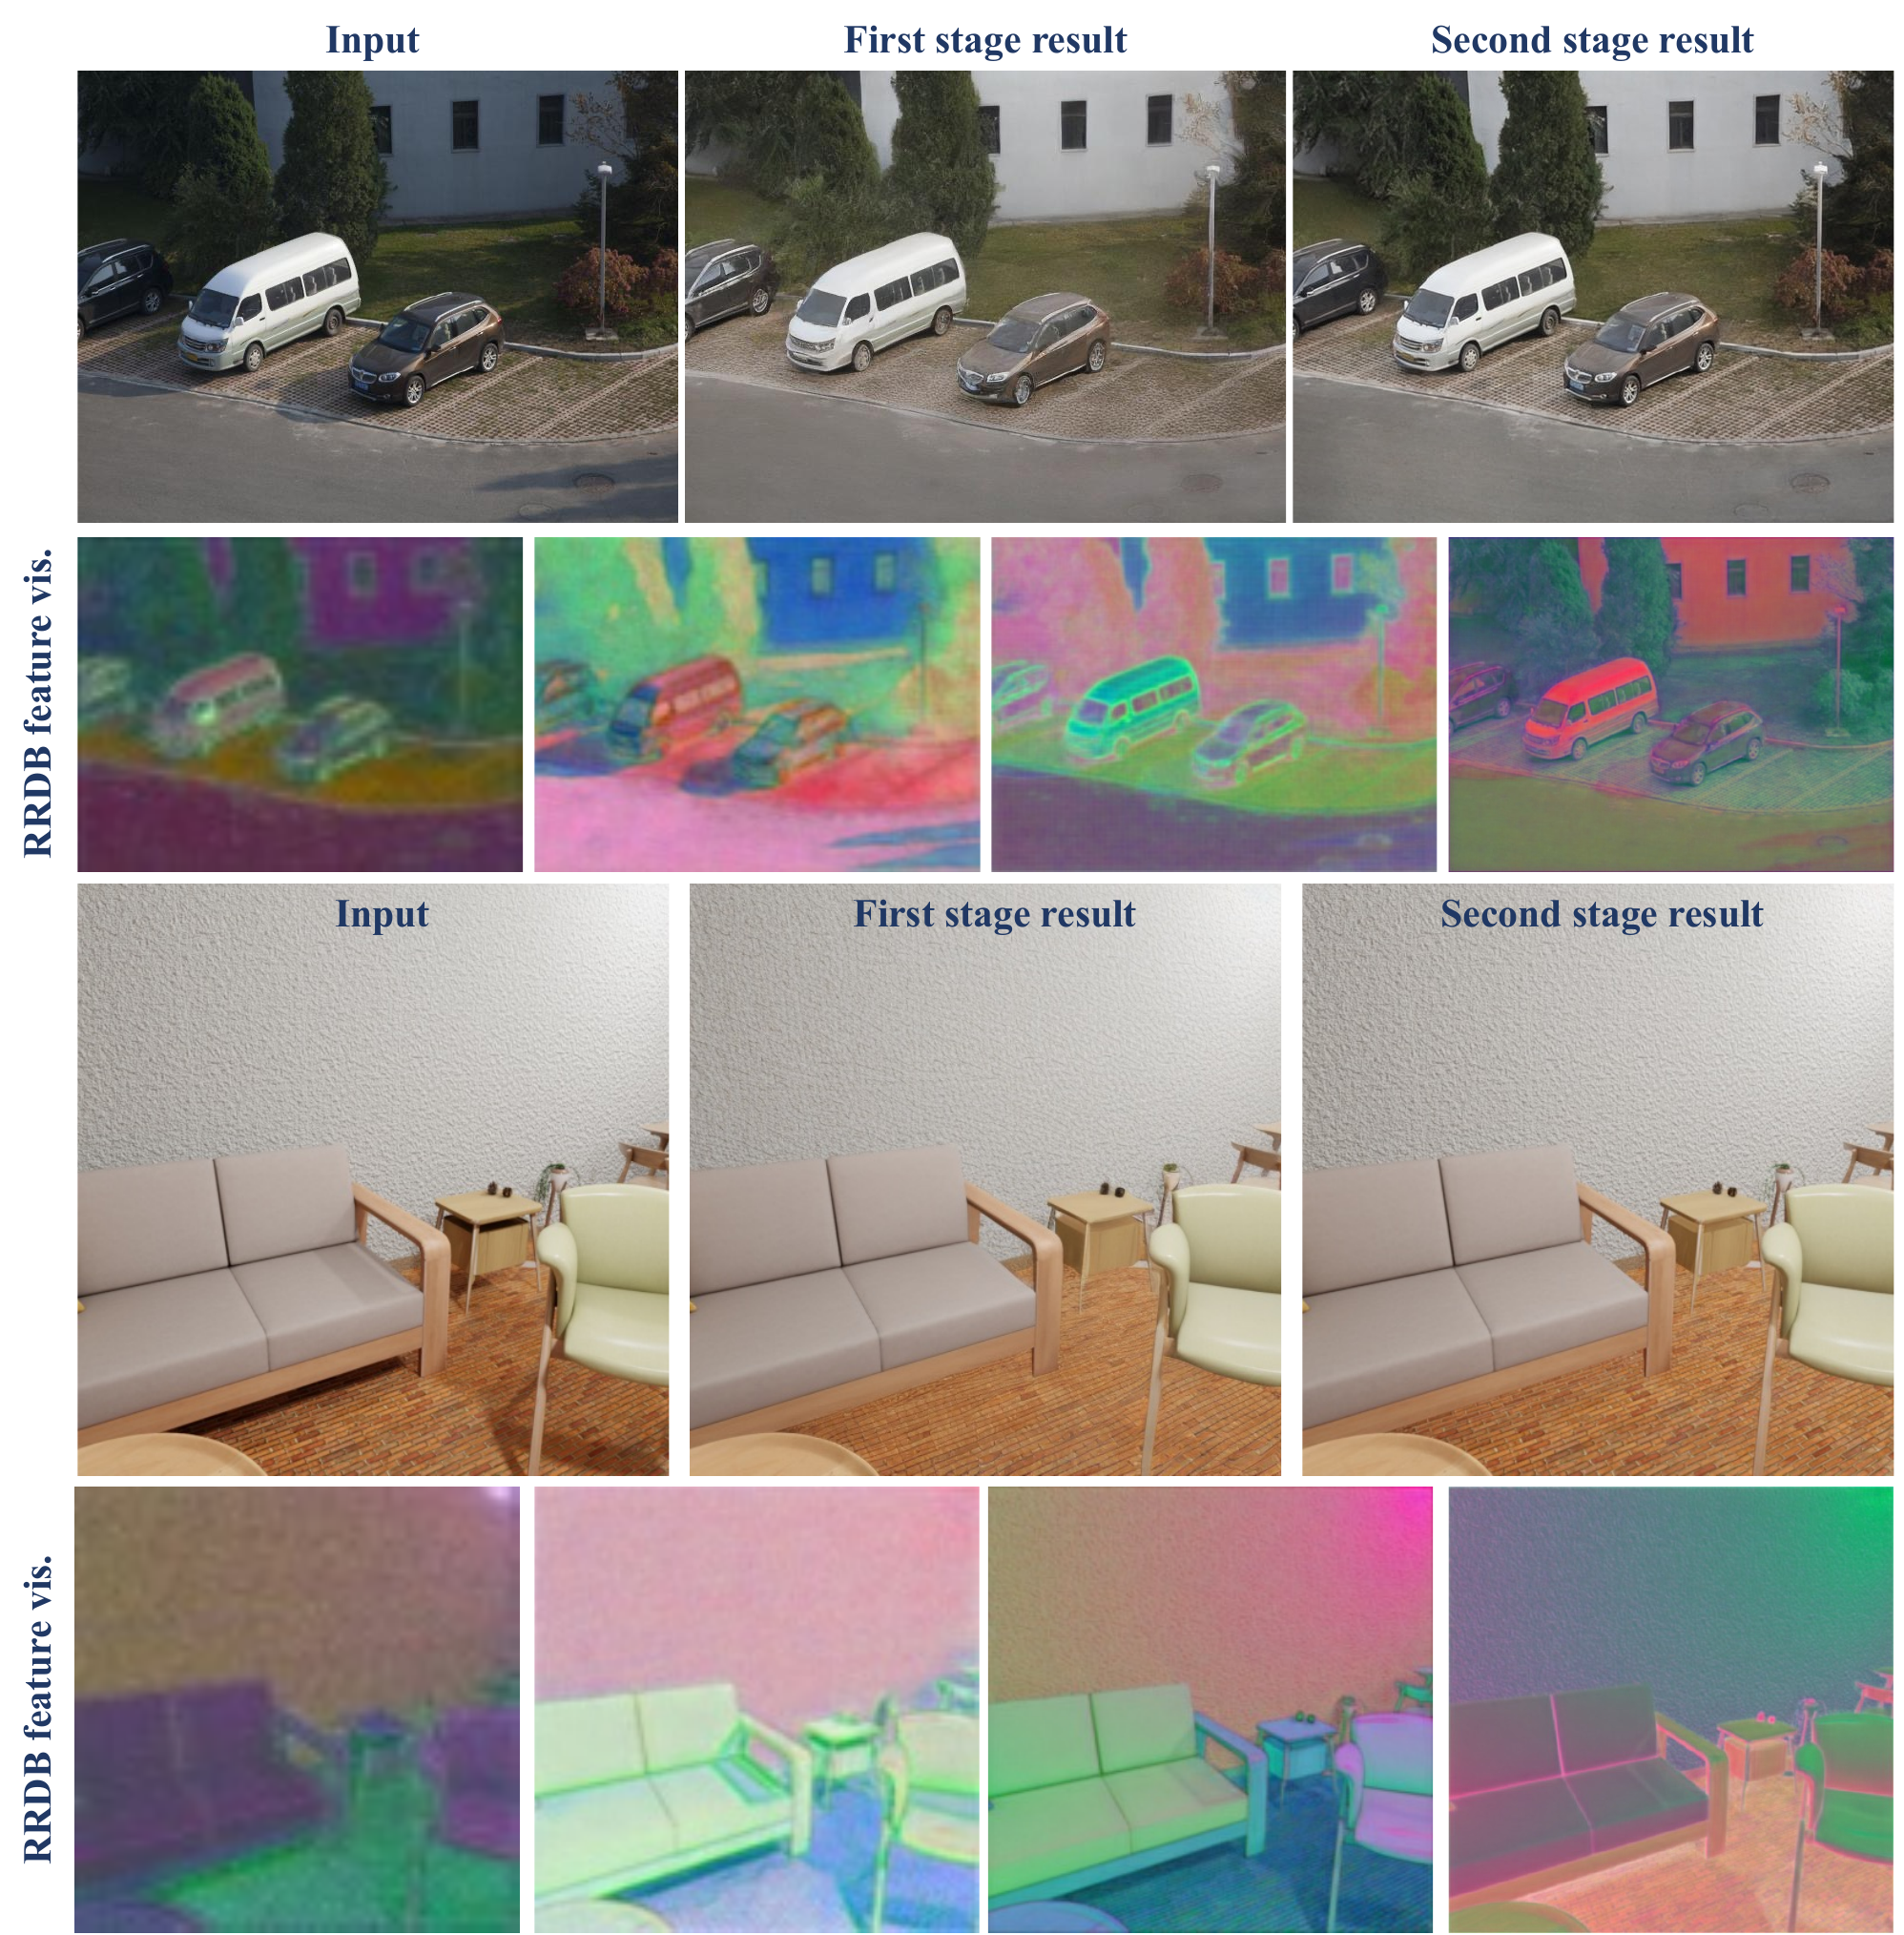}
\caption{\textbf{Additional results from our first and second stages, along with the visualization of RRDB features added to each decoder layer.}}
\label{fig:rrdb_vis} 
\end{figure*}

\subsection{More results from the cross-dataset evaluation}

As described in the main paper, we evaluate the generalizability of our method through cross-dataset testing. This includes training on ISTD+ and testing on SRD, training on SRD and testing on ISTD+, and training on INS (a synthetic dataset) while testing on WRSD+ (real-world captures). Notably, in both the ISTD+ and SRD datasets, the objects casting shadows in the training and testing splits are limited and often quite similar—such as the umbrellas shown in the third and fourth rows of Fig.~\ref{fig:supp_cross_dataset}. Therefore, cross-dataset evaluation provides a more robust demonstration of each method.

As shown in Fig.~\ref{fig:supp_cross_dataset}, when tested on a different dataset, methods like Refusion~\cite{luo2023refusion}, ShadowDiffusion~\cite{guo2023shadowdiffusion}, DeS3~\cite{jin2024des3}, and OmniSR~\cite{xu2024omnisr} tend to leave residual shadows in their results. In contrast, our method achieves superior performance under this evaluation setting. Leveraging the generative priors of Stable Diffusion~\cite{rombach2022high}, our approach demonstrates strong generalizability to unseen shadow-casting objects and diverse background types, which is a critical requirement for practical real-world shadow-removal applications.

\subsection{Evaluation on fixed and unfixed VAE decoder}

In our second stage, we fixed the decoder parameters and modulated each layer's output features by incorporating features from the corresponding VAE encoder layer. In this section, we evaluate our method using an unfixed VAE decoder and compared it with the fixed version. The results revealed no significant differences between the two configurations (Table~\ref{tab:fix_unfixed}). Therefore, we chose the fixed VAE decoder version for its advantage in reducing memory usage.

\begin{table}[t]
\center
\begin{tabular}{c c c}
\hline
\multirow{2}{*}{Dataset} & ISTD+ & SRD \\
& PSNR$$/SSIM$$ & PSNR$$/SSIM$$ \\
\hline
Fixed VAE decoder & 35.19/0.974 & 33.63/0.968 \\
Unfixed VAE decoder & 35.18/0.974 & 33.69/0.969 \\
\hline
\end{tabular}
\caption{\textbf{Ablation study on fixed vs. unfixed VAE decoder.}}
\label{tab:fix_unfixed}
\end{table}

\subsection{Qualitative results of ablation studies}

We present the qualitative results of the ablation studies. As shown in Fig.~\ref{fig:supp_ablation}, our full model achieves the best shadow removal performance compared to the other ablation configurations. In the ``Wo/ DINO'' ablation, we observe that DINO features help reduce some shadows, indicating that it can help filter out shadow-free information and inject it into the VAE decoder features during our Detail Injection stage.

\begin{figure*}[t!]
\centering
\includegraphics[width=1.0\linewidth]{./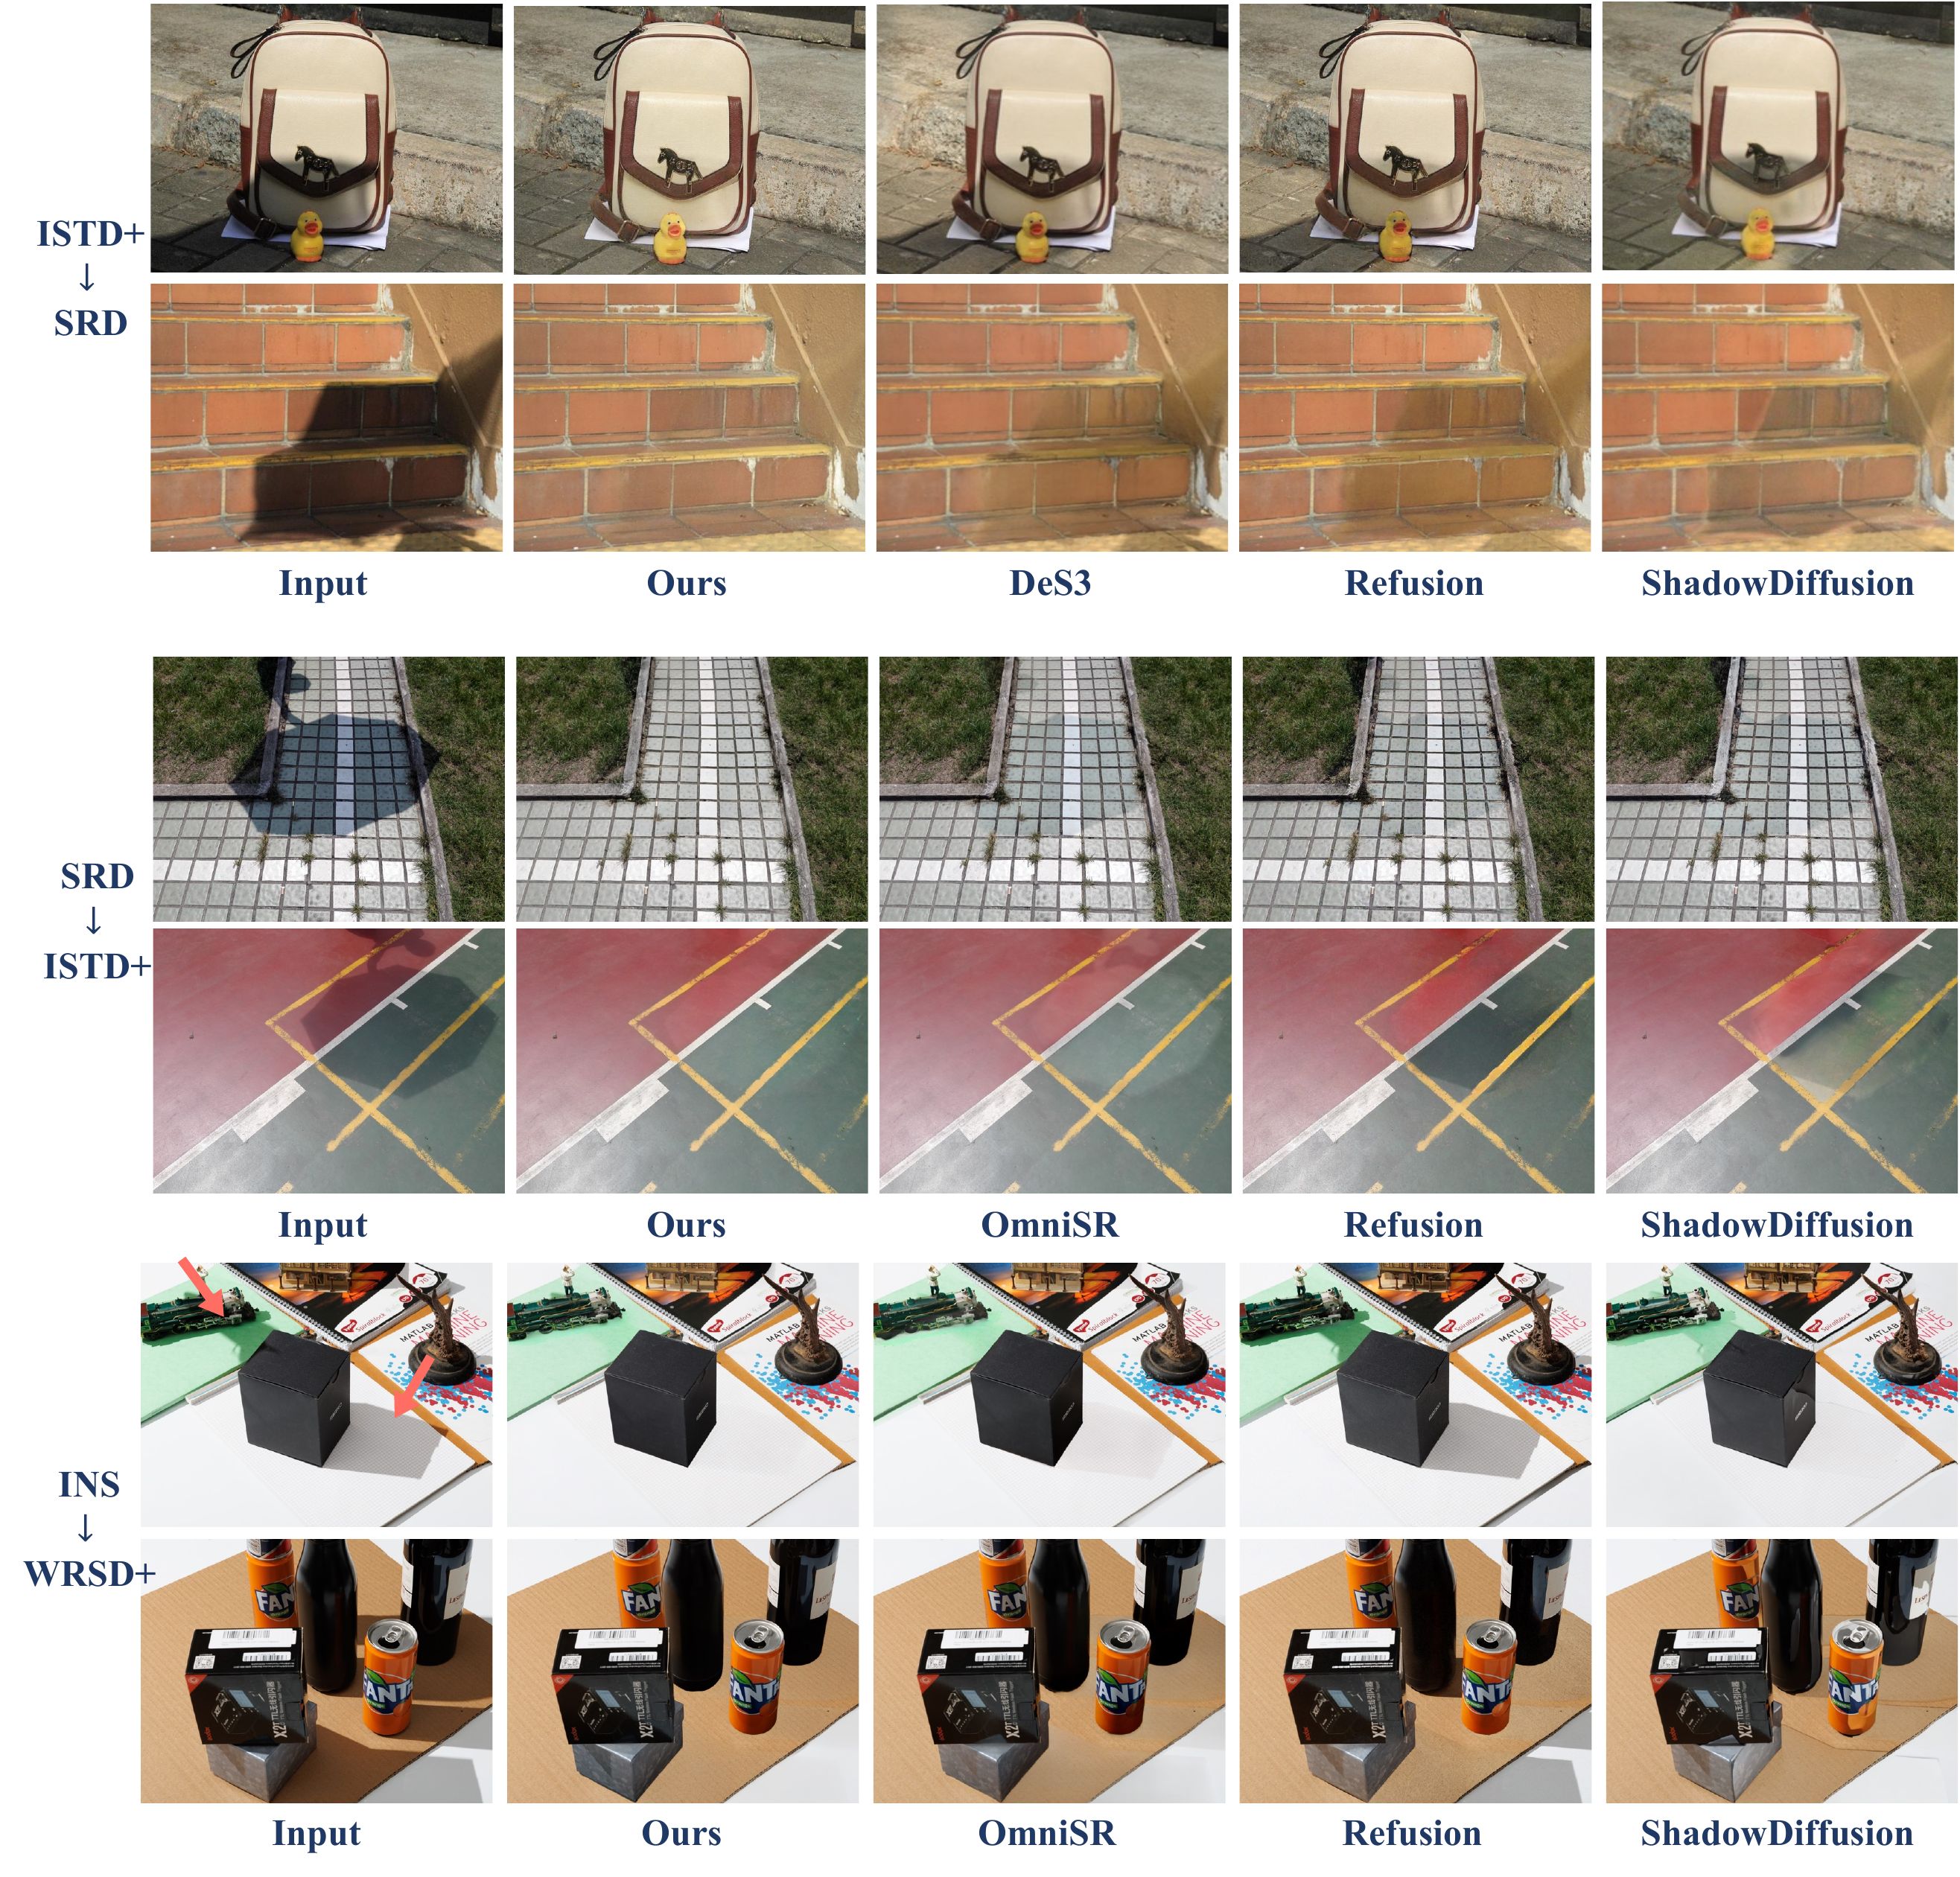}
\caption{\textbf{Additional results from our cross-dataset evaluation.}}
\label{fig:supp_cross_dataset} 
\end{figure*}

\begin{figure*}[t!]
\centering
\includegraphics[width=1.0\linewidth]{./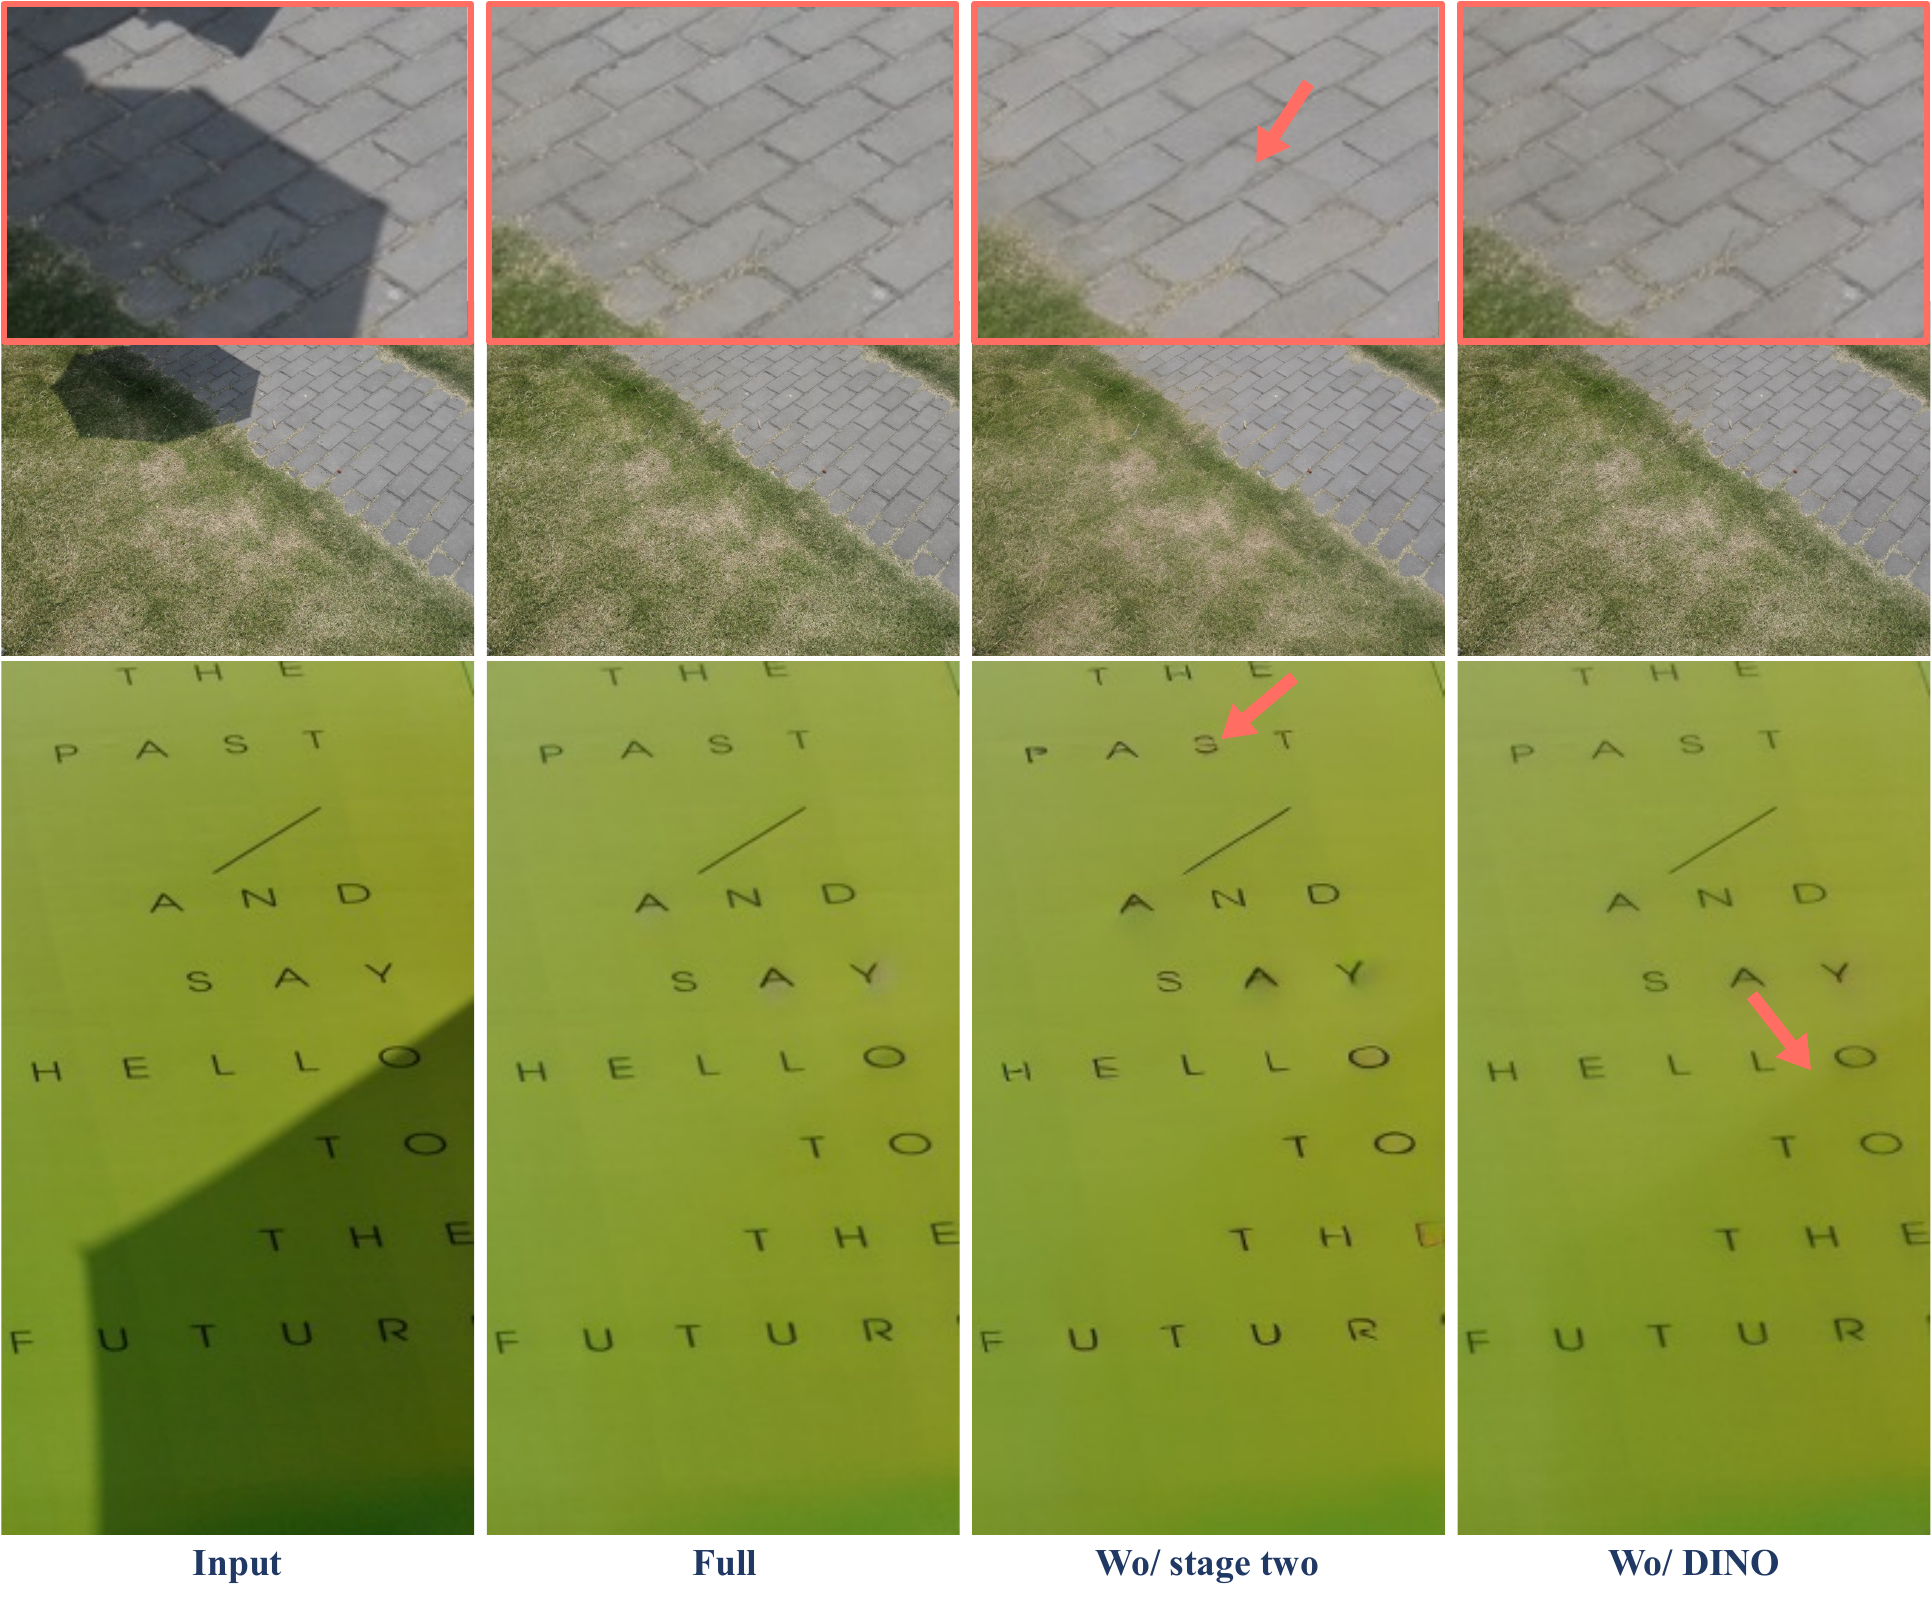}
\caption{\textbf{Qualitative results of ablation studies.}}
\label{fig:supp_ablation} 
\end{figure*}

% \subsection{Runing Time.}
